# Supplementary material for: Evidence for Phenylium Reactivity under Interstellar Relevant Conditions
Source: arXiv:2506.13290 source file (2026-03-26)
Supplement: Supplementary file 1 [file SI_Table.pdf]

|     | Reaction ( $k = \alpha \times (T/300)^\beta \exp(-\gamma/T)$ )                                         | $\alpha$                         | $\beta$                 | $\gamma$    | ref                                                                                                              |
|-----|--------------------------------------------------------------------------------------------------------|----------------------------------|-------------------------|-------------|------------------------------------------------------------------------------------------------------------------|
| 1.  | $H_3^+ + C_6H_4 \rightarrow C_6H_5^+ + H_2$                                                            | 3.90E-09                         | -0.5                    | 0           | / $H_3^+ + C_6H_6$                                                                                               |
| 2.  | $H_3^+ + l-C_6H_4 \rightarrow C_6H_5^+ + H_2$                                                          | 3.90E-09                         | 0                       | 0           | / $H_3^+ + C_6H_6$                                                                                               |
| 3.  | $H_3^+ + C_6H_6 \rightarrow C_6H_7^+ + H_2$                                                            | 3.90E-09                         | 0                       | 0           | <sup>1</sup>                                                                                                     |
| 4.  | $H_3^+ + l-C_6H_6 \rightarrow l-C_3H_3^+ + CH_3CCH + H_2$                                              | 3.90E-09                         | -0.5                    | 0           | / $H_3^+ + C_6H_6$                                                                                               |
| 5.  | $H_3^+ + C_7H_5 \rightarrow C_6H_7^+ + CH_2$                                                           | 3.90E-09                         | 0                       | 0           | / $H_3^+ + C_6H_6$                                                                                               |
| 6.  | $l-C_3H_3^+ + l-C_3H \rightarrow C_6H_4^+ + H_2$<br>$\rightarrow C_6H_5^+ + H$                         | 1.00E-09<br>1.00E-09             | -0.5<br>-0.5            | 0<br>0      | / $l-C_3H_3^+ + C_2H_2$ , $l-C_3H_3^+ + C_2H_4$ <sup>2</sup>                                                     |
| 7.  | $C_3H_4^+ + CH_3CCH \rightarrow C_6H_7^+ + H$<br>$\rightarrow C_3H_5^+ + C_3H_3$                       | 7.50E-10<br>3.50E-10             | -0.5<br>-0.5            | 0<br>0      | <sup>2, 3, 4</sup>                                                                                               |
| 8.  | $C_3H_4^+ + CH_2CCH_2 \rightarrow C_6H_7^+ + H$<br>$\rightarrow C_3H_5^+ + C_3H_3$                     | 8.00E-10<br>3.00E-10             | 0<br>0                  | 0<br>0      | <sup>2, 3</sup>                                                                                                  |
| 9.  | $C_3H_5^+ + CH_3CCH \rightarrow C_6H_7^+ + H_2$                                                        | 7.00E-10                         | -0.5                    | 0           | <sup>5</sup>                                                                                                     |
| 10. | $C_3H_5^+ + CH_2CCH_2 \rightarrow C_6H_7^+ + H_2$                                                      | 7.00E-10                         | 0                       | 0           | / $C_3H_5^+ + CH_3CCH$                                                                                           |
| 11. | $C_4H_2^+ + C_2H_4 \rightarrow C_6H_5^+ + H$<br>$\rightarrow C_6H_4^+ + H_2$                           | 8.00E-10<br>2.00E-10             | 0<br>0                  | 0<br>0      | <sup>4</sup>                                                                                                     |
| 12. | $C_4H_3^+ + C_2H_2 \rightarrow l-C_6H_5^+ + h\nu$                                                      | 2.20E-10                         | 0                       | 0           | See text                                                                                                         |
| 13. | $C_4H_3^+ + C_2H_4 \rightarrow C_6H_5^+ + H_2$                                                         | 1.20E-10                         | 0                       | 0           | <sup>4</sup>                                                                                                     |
| 14. | $C_3H_5^+ + C_2H_2 \rightarrow C_7H_7^+ + h\nu$<br>$\rightarrow C_6H_5CH_2^+ + h\nu$                   | 1.60E-11<br>1.60E-11             | -0.5<br>-0.5            | 0<br>0      | <sup>4, 5, 6</sup>                                                                                               |
| 15. | $C_6H_5^+ + H_2 \rightarrow C_6H_7^+ + h\nu$                                                           | 6.00E-11                         | 0                       | 0           | <sup>7, 8, 9, 10, 11, 12</sup>                                                                                   |
| 16. | $N_2H^+ + C_6H_6 \rightarrow C_6H_7^+ + N_2$                                                           | 1.60E-09                         | 0                       | 0           | <sup>13</sup>                                                                                                    |
| 17. | $HCO^+ + C_6H_4 \rightarrow C_6H_5^+ + CO$                                                             | 1.60E-09                         | 0                       | 0           | $HCO^+ + C_6H_6$                                                                                                 |
| 18. | $HCO^+ + l-C_6H_4 \rightarrow l-C_6H_5^+ + CO$                                                         | 1.60E-09                         | -0.5                    | 0           | $HCO^+ + C_6H_6$                                                                                                 |
| 19. | $HCO^+ + C_6H_6 \rightarrow C_6H_7^+ + CO$                                                             | 1.60E-09                         | 0                       | 0           | <sup>13</sup>                                                                                                    |
| 20. | $H + C_6H_5 \rightarrow C_6H_6 + h\nu$                                                                 | 1.00E-10                         | 0                       | 0           | <sup>14</sup>                                                                                                    |
| 21. | $C + C_6H_6 \rightarrow C_7H_5 + H$                                                                    | 3.00E-10                         | 0                       | 0           | <sup>15, 16</sup>                                                                                                |
| 22. | $C + C_6H_5C_2H \rightarrow C_6H_6 + C_3$                                                              | 3.00E-10                         | 0                       | 0           | / $C + C_6H_6$ , arbitrary branching ratio                                                                       |
| 23. | $C_2H + C_2H_3C_2H \rightarrow l-C_6H_4 + H$                                                           | 2.00E-10                         | 0                       | 0           | / $C_2H + C_4H_2$ <sup>17</sup> , $C_2H + C_4H_6$ <sup>18</sup>                                                  |
| 24. | $C_2H + CH_2CHCHCH_2 \rightarrow l-C_6H_6 + H$                                                         | 2.00E-10                         | 0                       | 0           | <sup>18</sup>                                                                                                    |
| 25. | $C_2H + C_6H_6 \rightarrow C_6H_5C_2H + H$                                                             | 3.28E-10                         | -0.18                   | 0           | <sup>19, 20</sup>                                                                                                |
| 26. | $C_2H_3 + C_4H_3 \rightarrow C_6H_5 + H$                                                               | 4.00E-11                         | 0                       | 0           | <sup>21</sup> , linear $l-C_6H_5$ isomers may also be produced.                                                  |
| 27. | $C_3H_3 + C_3H_3 \rightarrow C_6H_6 + h\nu$                                                            | 6.50E-11                         | 0                       | 0           | <sup>22, 23</sup> other $C_6H_6$ isomers may also be produced and the $H + C_6H_5$ pathway may not be negligible |
| 28. | $CN + C_6H_6 \rightarrow C_6H_5CN + H$                                                                 | 4.00E-10                         | 0                       | 0           | <sup>24</sup>                                                                                                    |
| 29. | $C_6H_5^+ + e^- \rightarrow C_6H_4 + H$<br>$\rightarrow C_6H_2 + H + H_2$                              | 2.00E-07<br>1.00E-06             | -0.3<br>-0.3            | 0           | rate from <sup>25</sup>                                                                                          |
| 30. | $l-C_6H_5^+ + e^- \rightarrow C_6H_4 + H$<br>$\rightarrow C_6H_2 + H + H_2$                            | 1.00E-06<br>1.00E-06             | -0.3<br>-0.3            | 0           | / $C_6H_5^+ + e^-$                                                                                               |
| 31. | $C_6H_6^+ + e^- \rightarrow C_6H_5 + H$<br>$\rightarrow C_6H_4 + H_2$<br>$\rightarrow C_3H_3 + C_3H_3$ | 1.00E-06<br>1.00E-07<br>1.00E-07 | -0.69<br>-0.69<br>-0.69 | 0<br>0<br>0 | rate constant from <sup>26</sup> , branching ratio guessed by comparison with $C_6H_6$ photodissociation         |
| 32. | $C_6H_7^+ + e^- \rightarrow C_6H_6 + H$<br>$\rightarrow C_6H_4 + H_2$<br>$\rightarrow C_6H_5 + H + H$  | 2.00E-06<br>1.00E-07<br>1.00E-07 | -0.83<br>-0.83<br>-0.83 | 0<br>0<br>0 | Global rate from <sup>26</sup>                                                                                   |

|     |                                                                                                                 |          |       |   |                                                                                                                                                                                                                                                                                                                                                          |
|-----|-----------------------------------------------------------------------------------------------------------------|----------|-------|---|----------------------------------------------------------------------------------------------------------------------------------------------------------------------------------------------------------------------------------------------------------------------------------------------------------------------------------------------------------|
| 33. | $\text{C}_6\text{H}_5\text{CH}_2^+ + \text{e}^- \rightarrow \text{C}_6\text{H}_5 + \text{CH}_2$                 | 3.00E-07 | -0.70 | 0 | rate from <sup>25, 27</sup> , arbitrary branching ratios                                                                                                                                                                                                                                                                                                 |
|     | $\rightarrow \text{C}_6\text{H}_6 + \text{CH}$                                                                  | 3.00E-07 | -0.70 | 0 |                                                                                                                                                                                                                                                                                                                                                          |
|     | $\rightarrow \text{CH}_3\text{CCH} + \text{C}_4\text{H}_2 + \text{H}$                                           | 1.00E-07 | -0.70 | 0 |                                                                                                                                                                                                                                                                                                                                                          |
|     | $\rightarrow \text{CH}_2\text{CCH}_2 + \text{C}_4\text{H}_2 + \text{H}$                                         | 1.00E-07 | -0.70 | 0 |                                                                                                                                                                                                                                                                                                                                                          |
| 34. | $\text{C}_7\text{H}_7^+ + \text{e}^- \rightarrow \text{C}_6\text{H}_5 + \text{CH}_2$                            | 3.00E-07 | -0.70 | 0 | rate from <sup>25, 27</sup> , arbitrary branching ratios                                                                                                                                                                                                                                                                                                 |
|     | $\rightarrow \text{C}_6\text{H}_6 + \text{CH}$                                                                  | 3.00E-07 | -0.70 | 0 |                                                                                                                                                                                                                                                                                                                                                          |
|     | $\rightarrow \text{CH}_3\text{CCH} + \text{C}_4\text{H}_2 + \text{H}$                                           | 1.00E-07 | -0.70 | 0 |                                                                                                                                                                                                                                                                                                                                                          |
|     | $\rightarrow \text{CH}_2\text{CCH}_2 + \text{C}_4\text{H}_2 + \text{H}$                                         | 1.00E-07 | -0.70 | 0 |                                                                                                                                                                                                                                                                                                                                                          |
| 35. | $\text{C}_6\text{H}_5\text{CCH}_2^+ + \text{e}^- \rightarrow \text{C}_6\text{H}_5\text{C}_2\text{H} + \text{H}$ | 1.00E-06 | -0.83 | 0 | /C <sub>6</sub> H <sub>6</sub> <sup>+</sup> + e <sup>-</sup> and C <sub>6</sub> H <sub>5</sub> CH <sub>2</sub> <sup>+</sup> /C <sub>7</sub> H <sub>7</sub> <sup>+</sup> + e <sup>-</sup> . Large uncertainties, C <sub>6</sub> H <sub>6</sub> + C <sub>2</sub> H and C <sub>6</sub> H <sub>5</sub> + C <sub>2</sub> H <sub>2</sub> may also be produced. |
| 36. | $\text{C}_6\text{H}_5\text{CNH}^+ + \text{e}^- \rightarrow \text{C}_6\text{H}_5\text{CN} + \text{H}$            | 1.50E-06 | -0.83 | 0 | /C <sub>6</sub> H <sub>6</sub> <sup>+</sup> + e <sup>-</sup> , C <sub>6</sub> H <sub>5</sub> CH <sub>2</sub> <sup>+</sup> /C <sub>7</sub> H <sub>7</sub> <sup>+</sup> + e <sup>-</sup> and HC <sub>3</sub> NH <sup>+</sup> + e <sup>-</sup>                                                                                                              |
|     | $\rightarrow \text{C}_6\text{H}_5 + \text{HCN}$                                                                 | 5.00E-07 | -0.83 | 0 |                                                                                                                                                                                                                                                                                                                                                          |
|     | $\rightarrow \text{C}_6\text{H}_6 + \text{HCN}$                                                                 | 5.00E-07 | -0.83 | 0 |                                                                                                                                                                                                                                                                                                                                                          |

1. Milligan DB, Wilson PF, Freeman CG, Meot-Ner M, McEwan MJ. Dissociative Proton Transfer Reactions of H<sub>3</sub><sup>+</sup>, N<sub>2</sub>H<sup>+</sup>, and H<sub>3</sub>O<sup>+</sup> with Acyclic, Cyclic, and Aromatic Hydrocarbons and Nitrogen Compounds, and Astrochemical Implications<sup>†</sup>. *The Journal of Physical Chemistry A* 2002, **106**(42): 9745-9755.
2. Anicich VG. An index of the literature for bimolecular gas phase cation-molecule reaction kinetics. *JPL Publication-03-19, Pasadena, CA, USA* 2003.
3. Anicich VG, Wilson P, McEwan MJ. Termolecular ion-molecule reactions in Titan's atmosphere. IV. A search made at up to 1 micron in pure hydrocarbons. *Journal of the American Society for Mass Spectrometry* 2003, **14**(8): 900-915.
4. McEwan MJ, Anicich VG. Titan's ion chemistry: A laboratory perspective. *Mass Spectrometry Reviews* 2007, **26**(2): 281-319.
5. Anicich VG, Wilson PF, McEwan MJ. An ICR Study of Ion-Molecules Reactions Relevant to Titan Atmosphere: An Investigation of Binary Hydrocarbon Mixtures up to 1 Micron. *Journal of the American Society for Mass Spectrometry* 2006, **17**(4): 544-561.
6. Ozturk F, Moini M, Brill FW, Eyler JR, Buckley TJ, Lias SG, *et al.* Reactions of C<sub>5</sub>H<sub>3</sub><sup>+</sup> and C<sub>5</sub>H<sub>5</sub><sup>+</sup> ions with acetylene and diacetylene. *The Journal of Physical Chemistry* 1989, **93**(10): 4038-4044.
7. Ausloos P, Lias SG, Buckley TJ, Rogers EE. Concerning the formation and the kinetics of phenylium ions. *International Journal of Mass Spectrometry and Ion Processes* 1989, **92**(0): 65-77.
8. Petrie S, Javahery G, Bohme DK. Gas-phase reactions of benzenoid hydrocarbon ions with hydrogen atoms and molecules: uncommon constraints to reactivity. *Journal of the American Chemical Society* 1992, **114**(23): 9205-9206.
9. Scott GBI, Fairley DA, Freeman CG, McEwan MJ, Adams NG, Babcock LM. CmHn<sup>+</sup> Reactions with H and H<sub>2</sub>: An Experimental Study. *The Journal of Physical Chemistry A* 1997, **101**(27): 4973-4978.
10. Snow TP, Le Page V, Keheyan Y, Bierbaum VM. The interstellar chemistry of PAH cations. *Nature* 1998, **391**(6664): 259-260.
11. McEwan M, J., Scott G, B. I., Adams N, G., Babcock L, M., Terzieva R, Herbst E. New H and H<sub>2</sub> Reactions with Small Hydrocarbon Ions and Their Roles in Benzene Synthesis in Dense Interstellar Clouds. *The Astrophysical Journal* 1999, **513**(1): 287.
12. Keheyan Y. A Fourier-transform ion-cyclotron-resonance study of the reactions of polycyclic aromatic hydrocarbon cations with molecules of interstellar interest. *Chemical Physics Letters* 2001, **340**(5): 405-412.
13. Wakelam V, Gratier P, Loison J-C, Hickson KM, Penguen J, Mechineau A. The 2024 KIDA network for interstellar chemistry. *A&A* 2024, **689**: A63.
14. Vuitton V, Yelle RV, Lavvas P, Klippenstein SJ. Rapid Association Reactions at Low Pressure: Impact on the Formation of Hydrocarbons on Titan. *The Astrophysical Journal* 2012, **744**(1): 11.

15. Bettinger HF, Schleyer PVR, Schaefer III HF, Schreiner PR, Kaiser RI, Lee YT. Reaction of benzene with a ground state carbon atom, C(3Pj). *Journal of Chemical Physics* 2000, **113**(10): 4250-4264.
16. Bergeat A, Loison J-C. Reaction of carbon atoms, C (2p2, 3P) with C<sub>2</sub>H<sub>2</sub>, C<sub>2</sub>H<sub>4</sub> and C<sub>6</sub>H<sub>6</sub>: Overall rate constant and relative atomic hydrogen production. *Physical Chemistry Chemical Physics* 2001, **3**(11): 2038-2042.
17. Landera A, Krishtal SP, Kislov VV, Mebel AM, Kaiser RI. Theoretical study of the C<sub>6</sub>H<sub>3</sub> potential energy surface and rate constants and product branching ratios of the C<sub>2</sub>H+C<sub>4</sub>H<sub>2</sub> and C<sub>4</sub>H+C<sub>2</sub>H<sub>2</sub> reactions. *The Journal of Chemical Physics* 2008, **128**(21).
18. Jones BM, Zhang F, Kaiser RI, Jamal A, Mebel AM, Cordiner MA, *et al.* Formation of benzene in the interstellar medium. *Proceedings of the National Academy of Sciences* 2011, **108**(2): 452.
19. Woon DE. Modeling chemical growth processes in Titan's atmosphere: 1. Theoretical rates for reactions between benzene and the ethynyl (C<sub>2</sub>H) and cyano (CN) radicals at low temperature and pressure. *Chemical Physics* 2006, **331**(1): 67-76.
20. Goulay F, Leone SR. Low-Temperature Rate Coefficients for the Reaction of Ethynyl Radical (C<sub>2</sub>H) with Benzene. *The Journal of Physical Chemistry A* 2006, **110**(5): 1875-1880.
21. Duran RP, Amorebieta VT, Colussi AJ. Is the homogeneous thermal dimerization of acetylene a free-radical chain reaction? Kinetic and thermochemical analysis. *The Journal of Physical Chemistry* 1988, **92**(3): 636-640.
22. Miller JA, Klippenstein SJ. The Recombination of Propargyl Radicals and Other Reactions on a C<sub>6</sub>H<sub>6</sub> Potential. *The Journal of Physical Chemistry A* 2003, **107**(39): 7783-7799.
23. Vuitton V, Yelle RV, Klippenstein SJ, Hörst SM, Lavvas P. Simulating the density of organic species in the atmosphere of Titan with a coupled ion-neutral photochemical model. *Icarus* 2019, **324**: 120-197.
24. Trevitt AJ, Goulay F, Taatjes CA, Osborn DL, Leone SR. Reactions of the CN Radical with Benzene and Toluene: Product Detection and Low-Temperature Kinetics. *The Journal of Physical Chemistry A* 2009, **114**(4): 1749-1755.
25. Fournier JA, Shuman NS, Melko JJ, Ard SG, Viggiano AA. A novel technique for measurement of thermal rate constants and temperature dependences of dissociative recombination: CO<sub>2</sub><sup>+</sup>, CF<sub>3</sub><sup>+</sup>, N<sub>2</sub>O<sup>+</sup>, C<sub>7</sub>H<sub>8</sub><sup>+</sup>, C<sub>7</sub>H<sub>7</sub><sup>+</sup>, C<sub>6</sub>H<sub>6</sub><sup>+</sup>, C<sub>6</sub>H<sub>5</sub><sup>+</sup>, C<sub>5</sub>H<sub>6</sub><sup>+</sup>, C<sub>4</sub>H<sub>4</sub><sup>+</sup>, and C<sub>3</sub>H<sub>3</sub><sup>+</sup>. *The Journal of Chemical Physics* 2013, **138**(15).
26. Hamberg M, Vigren E, Thomas RD, Zhaunerchyk V, Zhang M, Trippel S, *et al.* Experimental studies of the dissociative recombination processes for the C<sub>6</sub>D<sub>6</sub><sup>+</sup> and C<sub>6</sub>D<sub>7</sub><sup>+</sup> ions. *EAS Publications Series* 2011, **46**: 241-249.
27. Rebrion-Rowe C, Mostefaoui T, Laubé S, Mitchell JBA. The dissociative recombination of hydrocarbon ions. III. Methyl-substituted benzene ring compounds. *The Journal of Chemical Physics* 2000, **113**(8): 3039-3045.
